# Supplementary material for: Invertible Denoising Network: A Light Solution for Real Noise Removal
Source: arXiv:2104.10546 source file (2021-04-21)
Supplement: Supplementary file 1 [file fig_sidd.tex]

\setcounter{page}{1}

% \begin{center}
% {\LARGE\bfseries Supplementary Materials}

% {\Large Invertible Denoising Network: A Light Solution for Real Noise Removal}
% \end{center}

\begin{figure*}
\vspace{4mm}
\centering
\begin{subfigure}{1.\textwidth} 
  \centering
    \includegraphics[width=.16\linewidth]{CVPR2021/supp/z_hf/0_noisy.png}
    \includegraphics[width=.16\linewidth]{CVPR2021/supp/z_hf/0_clean.png}
    \includegraphics[width=.16\linewidth]{CVPR2021/supp/z_hf/2.png}
    \includegraphics[width=.16\linewidth]{CVPR2021/supp/z_hf/3.png}
    \includegraphics[width=.16\linewidth]{CVPR2021/supp/z_hf/4.png}   \includegraphics[width=.16\linewidth]{CVPR2021/supp/z_hf/5.png}
  % figure 1
%   \caption{\textbf{DND~\cite{DND_2017_CVPR} visualization examples.} \ourmodel produces fewer fake dots, restores better colors and finer textures. }
  \label{fig:sub-first}
\end{subfigure}
% Caption
\begin{subfigure}{.16\textwidth}
  \centering
  % include first image
  \caption{Noisy}
  \label{subfig: Noisy}
\end{subfigure}
\begin{subfigure}{.16\textwidth}
  \centering
  \captionsetup{justification=centering}
  % include second image
  \caption{Denoised ($z_\text{HF}^1$) \\ PSNR: 34.528 dB}
  \label{subfig: z_hf_1}
\end{subfigure}
\begin{subfigure}{.16\textwidth}
  \centering
  \captionsetup{justification=centering}
  % include second image
  \caption{$z_\text{HF}^2$ \\ PSNR: 34.522 dB}
  \label{subfig: z_hf_2}
\end{subfigure}
\begin{subfigure}{.16\textwidth}
  \centering
  \captionsetup{justification=centering}
  % include first image
  \caption{$z_\text{HF}^3$ \\ PSNR: 34.518 dB}
  \label{subfig: z_hf_3}
\end{subfigure}
\begin{subfigure}{.16\textwidth}
  \centering
  \captionsetup{justification=centering}
  % include second image
  \caption{$z_\text{HF}^4$ \\ PSNR: 34.523 dB}
  \label{subfig: z_hf_4}
\end{subfigure}
\begin{subfigure}{.16\textwidth}
  \centering
  \captionsetup{justification=centering}
  % include second image
  \caption{$z_\text{HF}^5$ \\ PSNR: 34.525 dB}
  \label{subfig: z_hf_5}
\end{subfigure}
% SIDD
%\vspace{-4mm}
\caption{The denoised results achieved with different $z_\text{HF}$ samples. The brighter regions in \autoref{subfig: z_hf_2}-\autoref{subfig: z_hf_5} illustrate the difference between the images restored with $z_\text{HF}^2$ - $z_\text{HF}^5$ and \autoref{subfig: z_hf_1}. The difference has been highlighted for better visualization. Best viewed in color on a high-resolution display. The major difference lies in the high-frequency regions such as edges and textures.}
\label{fig:zhf}
% \vspace{-6mm}
\end{figure*}

\section{Introduction}
In this section of the paper, first, we provide information about restoration using different $\zhf$ Samples. Next, we show how noise is generated with different $\z$, and finally, we provide more qualitative results of our network against state-of-the-art algorithms.

\section{Restore with Different $\zhf$ Samples}
In \autoref{fig:zhf}, we present the restored clean images with different $\zhf^{i}$ samples. Different $i$ represent distinct sampled $\zhf$. The quantitative difference between different denoised images is no more than 0.01 dB. In  \autoref{subfig: z_hf_2}-\autoref{subfig: z_hf_5}, we highlight the difference between the restored images of $\zhf^{i}$ ($i >= 2$) and the reconstructed image of $\zhf^{1}$. We observe that the major difference lies in the high-frequency regions, such as edges and textures.

% The qualitative difference between the images restored with different $\zhf^{i}$ and $\zhf^1$ is highlighted in the brighter regions in \autoref{subfig: z_hf_2} - \autoref{subfig: z_hf_5}. From the images, we can observe that the main difference lies in the high-frequency regions such as edges and textures. 

\section{Generate Noise with Different $\z$}
As presented in Sec. 4.5, by introducing disturbances to $\z$, \ie, $\z' = \z + \epsilon \cdot \mathbf{v}$, we can reconstruct new noisy images.  Since the disturbances are small, we consider the original and the new generated noisy images follow the same distribution, supported by the low AKLD score in Tab. 5. Here, we study the influence of disturbance level $\epsilon$ and random sample $\mathbf{v}$. 

\vspace{4mm}
\noindent
\textbf{Different $\epsilon$ Levels.}
We generate new noisy images with different $\epsilon$ levels as described in Sec. 4.5. An example is shown in \autoref{fig:epsilon}. When $\epsilon=1 \times 10^{-3}$, artifacts can be observed in the generated noisy images. The visual results are better when $\epsilon=1 \times 10^{-4}$ and $1 \times 10^{-5}$. We observe that the difference is spatially variant and signal-dependent. When the disturbance is too small, such as $\epsilon=1 \times 10^{-6}$, the generated image visually shows no difference from the original one.

\vspace{10mm}
\noindent
\textbf{Different $\mathbf{v}$ Samples.}
We also present the generated noisy images with fixing $\epsilon = 1 \times 10^{-4}$ in \autoref{fig:z}. We introduce different disturbances to $\z$. Specifically, we sample $\mathbf{v}$ multiple times, obtaining $\{ \mathbf{v}_i \}_{i=1}^{N}$. For each $\mathbf{v}_i$, we obtain $\z_i = \z + \epsilon \cdot \mathbf{v}_i$. We can reconstruct a new noisy image for every $\z_i$. 

\section{More Qualitative Results}
\autoref{fig:more_sidd} and \autoref{fig:more_dnd} illustrate more qualitative results of \ourmodel against other competitive models. \ourmodel reconstructs sharp shapes, crisp edges, and clear textures. In comparison, other models produce blurry patterns and artifacts. 

%\clearpage

\begin{figure*}[t]
\centering
\begin{subfigure}{1.\textwidth} 
  \centering
    \includegraphics[width=.16\linewidth]{CVPR2021/supp/noise_increase_ep_0/noisy.PNG}   
    \includegraphics[width=.16\linewidth]{CVPR2021/supp/noise_increase_ep_0/contrast_9_281e-3.PNG}
    \includegraphics[width=.16\linewidth]{CVPR2021/supp/noise_increase_ep_0/contrast_9_281e-4.PNG}
    \includegraphics[width=.16\linewidth]{CVPR2021/supp/noise_increase_ep_0/contrast_9_281e-5.PNG}
    \includegraphics[width=.16\linewidth]{CVPR2021/supp/noise_increase_ep_0/contrast_9_281e-6.PNG}
  % figure 1
%   \caption{\textbf{DND~\cite{DND_2017_CVPR} visualization examples.} \ourmodel produces fewer fake dots, restores better colors and finer textures. }
  \label{fig:sub-first}
\end{subfigure}
% Caption
\begin{subfigure}{.16\textwidth}
  \centering
  % include first image
  \caption{Original Noisy}
  \label{subfig: Noisy}
\end{subfigure}
\begin{subfigure}{.16\textwidth}
  \centering
  \captionsetup{justification=centering}
  % include second image
  \caption{$\epsilon=1 \times 10^{-3}$}
  \label{subfig: 1e-3}
\end{subfigure}
\begin{subfigure}{.16\textwidth}
  \centering
  \captionsetup{justification=centering}
  % include second image
  \caption{$\epsilon=1 \times 10^{-4}$}
  \label{subfig: 1e-4}
\end{subfigure}
\begin{subfigure}{.16\textwidth}
  \centering
  \captionsetup{justification=centering}
  % include first image
  \caption{$\epsilon=1 \times 10^{-5}$}
  \label{subfig: 1e-5}
\end{subfigure}
\begin{subfigure}{.16\textwidth}
  \centering
  \captionsetup{justification=centering}
  % include first image
  \caption{$\epsilon=1 \times 10^{-6}$}
  \label{subfig: 1e-6}
\end{subfigure}
% SIDD
%\vspace{-4mm}
\caption{Noisy image generation with different $\epsilon$. \autoref{subfig: 1e-3} - \autoref{subfig: 1e-6} show the new generated noisy images with different disturbance levels to the noisy latent representation $\z$. The left part is the generated noisy image. The right part is the difference between the new noisy image and the original noisy one.}
\label{fig:epsilon}
\vspace{4mm}
\end{figure*}

\begin{figure*}
\centering
\begin{subfigure}{1.\textwidth} 
  \centering
    \includegraphics[width=.16\linewidth]{CVPR2021/supp/noise_gen_diff/orig_z_1.PNG}   
    \includegraphics[width=.16\linewidth]{CVPR2021/supp/noise_gen_diff/contrast_z_2.PNG}
    \includegraphics[width=.16\linewidth]{CVPR2021/supp/noise_gen_diff/contrast_z_3.PNG}
    \includegraphics[width=.16\linewidth]{CVPR2021/supp/noise_gen_diff/contrast_z_4.PNG}
    \includegraphics[width=.16\linewidth]{CVPR2021/supp/noise_gen_diff/contrast_z_5.PNG}
  % figure 1
  \label{fig:sub-first}
\end{subfigure}
\begin{subfigure}{1.\textwidth} 
  \centering
    \includegraphics[width=.16\linewidth]{CVPR2021/supp/noise_gen_diff/crop_z_1.PNG}   
    \includegraphics[width=.16\linewidth]{CVPR2021/supp/noise_gen_diff/crop_z_2.PNG}
    \includegraphics[width=.16\linewidth]{CVPR2021/supp/noise_gen_diff/crop_z_3.PNG}
    \includegraphics[width=.16\linewidth]{CVPR2021/supp/noise_gen_diff/crop_z_4.PNG}
    \includegraphics[width=.16\linewidth]{CVPR2021/supp/noise_gen_diff/crop_z_5.PNG}
  % figure 1
%   \caption{\textbf{DND~\cite{DND_2017_CVPR} visualization examples.} \ourmodel produces fewer fake dots, restores better colors and finer textures. }
  \label{fig:sub-second}
\end{subfigure}
% Caption
\begin{subfigure}{.16\textwidth}
  \centering
  % include first image
  \caption{Original Noisy}
  \label{subfig: Noisy}
\end{subfigure}
\begin{subfigure}{.16\textwidth}
  \centering
  \captionsetup{justification=centering}
  % include second image
  \caption{$\z_1$}
  \label{subfig: z1}
\end{subfigure}
\begin{subfigure}{.16\textwidth}
  \centering
  \captionsetup{justification=centering}
  % include second image
  \caption{$\z_2$}
  \label{subfig: z2}
\end{subfigure}
\begin{subfigure}{.16\textwidth}
  \centering
  \captionsetup{justification=centering}
  % include first image
  \caption{$\z_3$}
  \label{subfig: z3}
\end{subfigure}
\begin{subfigure}{.16\textwidth}
  \centering
  \captionsetup{justification=centering}
  % include first image
  \caption{$\z_4$}
  \label{subfig: z4}
\end{subfigure}
% SIDD
%\vspace{-4mm}
\caption{Noisy image generation with different $\z$ samples under $\epsilon=1 \times 10^{-4}$. The first rows of \autoref{subfig: z1} - \autoref{subfig: z4} show the generated new noisy images as well as the difference between the new generated ones and the original one. The second rows of \autoref{subfig: z1} - \autoref{subfig: z4} present the zoom-in difference between the patches from the generated noisy image and the original one.}
\label{fig:z}
% \vspace{-6mm}
\end{figure*}

\begin{figure*}[t]
\centering
% Caption
\begin{subfigure}{.16\textwidth}
  \centering
  % include first image
  \caption*{Noisy} 
\end{subfigure}
\begin{subfigure}{.16\textwidth}
  \centering
  % include second image
  \caption*{CBDNet~\cite{Guo2019Cbdnet}} 
\end{subfigure}
\begin{subfigure}{.16\textwidth}
  \centering
  % include second image
  \caption*{RIDNet~\cite{RIDNet}} 
\end{subfigure}
\begin{subfigure}{.16\textwidth}
  \centering
  % include first image
  \caption*{VDN~\cite{VDN}}   
\end{subfigure}
\begin{subfigure}{.16\textwidth}
  \centering
  % include second image
  \caption*{DANet~\cite{DANet}} 
\end{subfigure}
\begin{subfigure}{.16\textwidth}
  \centering
  % include second image
  \caption*{\ourmodel (Ours)} 
\end{subfigure}
% SIDD
\begin{subfigure}{1.\textwidth} 
  \centering
  % figure 1
  \includegraphics[width=.16\linewidth]{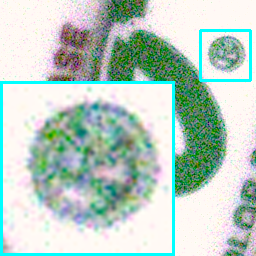} 
  \includegraphics[width=.16\linewidth]{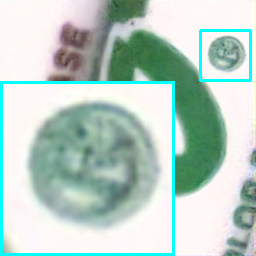} 
  \includegraphics[width=.16\linewidth]{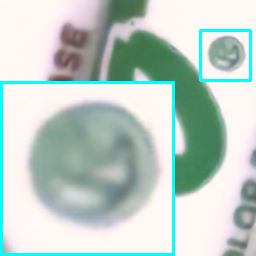} 
  \includegraphics[width=.16\linewidth]{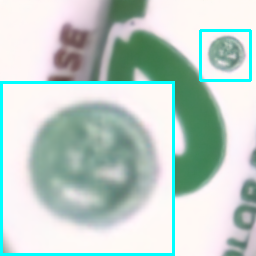}  
  \includegraphics[width=.16\linewidth]{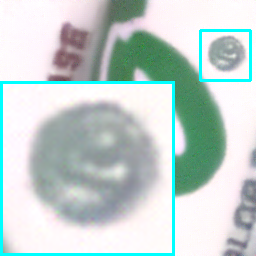}  
  \includegraphics[width=.16\linewidth]{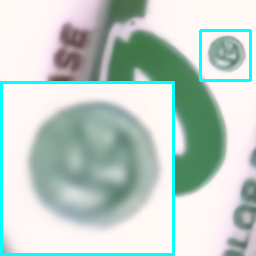} 
  % figure 2
  \includegraphics[width=.16\linewidth]{CVPR2021/supp/sidd_fig_1/box_noisy.PNG} 
  \includegraphics[width=.16\linewidth]{CVPR2021/supp/sidd_fig_1/box_cbdnet.PNG}  
  \includegraphics[width=.16\linewidth]{CVPR2021/supp/sidd_fig_1/box_ridnet.PNG} 
  \includegraphics[width=.16\linewidth]{CVPR2021/supp/sidd_fig_1/box_vdnet.PNG}  
  \includegraphics[width=.16\linewidth]{CVPR2021/supp/sidd_fig_1/box_danet.PNG}  
  \includegraphics[width=.16\linewidth]{CVPR2021/supp/sidd_fig_1/box_ours.PNG}  
  % figure 3
  \includegraphics[width=.16\linewidth]{CVPR2021/supp/sidd_fig_2/box_noisy.PNG} 
  \includegraphics[width=.16\linewidth]{CVPR2021/supp/sidd_fig_2/box_cbdnet.PNG}  
  \includegraphics[width=.16\linewidth]{CVPR2021/supp/sidd_fig_2/box_ridnet.PNG} 
  \includegraphics[width=.16\linewidth]{CVPR2021/supp/sidd_fig_2/box_vdnet.PNG}  
  \includegraphics[width=.16\linewidth]{CVPR2021/supp/sidd_fig_2/box_danet.PNG}  
  \includegraphics[width=.16\linewidth]{CVPR2021/supp/sidd_fig_2/box_ours.PNG}  
  % figure 4
  \includegraphics[width=.16\linewidth]{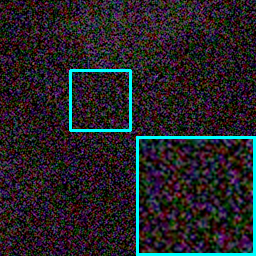} 
  \includegraphics[width=.16\linewidth]{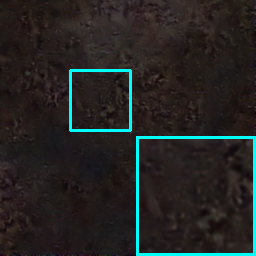}  
  \includegraphics[width=.16\linewidth]{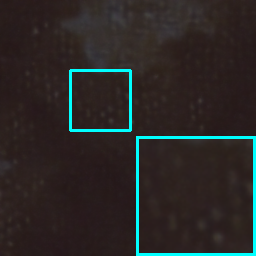} 
  \includegraphics[width=.16\linewidth]{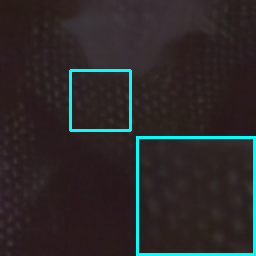}  
  \includegraphics[width=.16\linewidth]{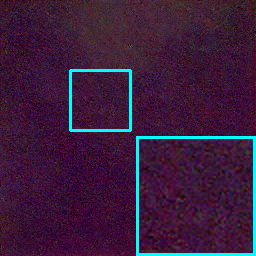}  
  \includegraphics[width=.16\linewidth]{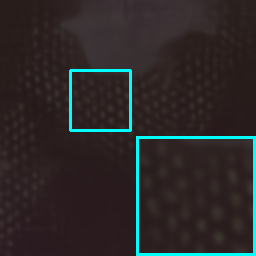}
  % figure 5
  \includegraphics[width=.16\linewidth]{CVPR2021/supp/sidd_fig_6/box_noisy.PNG} 
  \includegraphics[width=.16\linewidth]{CVPR2021/supp/sidd_fig_6/box_cbdnet.PNG}  
  \includegraphics[width=.16\linewidth]{CVPR2021/supp/sidd_fig_6/box_ridnet.PNG} 
  \includegraphics[width=.16\linewidth]{CVPR2021/supp/sidd_fig_6/box_vdnet.PNG}  
  \includegraphics[width=.16\linewidth]{CVPR2021/supp/sidd_fig_6/box_danet.PNG}  
  \includegraphics[width=.16\linewidth]{CVPR2021/supp/sidd_fig_6/box_ours.PNG}
  % figure 6
  \includegraphics[width=.16\linewidth]{CVPR2021/supp/sidd_fig_7/box_noisy.PNG} 
  \includegraphics[width=.16\linewidth]{CVPR2021/supp/sidd_fig_7/box_cbdnet.PNG}  
  \includegraphics[width=.16\linewidth]{CVPR2021/supp/sidd_fig_7/box_ridnet.PNG} 
  \includegraphics[width=.16\linewidth]{CVPR2021/supp/sidd_fig_7/box_vdnet.PNG}  
  \includegraphics[width=.16\linewidth]{CVPR2021/supp/sidd_fig_7/box_danet.PNG}  
  \includegraphics[width=.16\linewidth]{CVPR2021/supp/sidd_fig_7/box_ours.PNG}
  % figure 7
  \includegraphics[width=.16\linewidth]{CVPR2021/supp/sidd_fig_10/box_noisy.PNG} 
  \includegraphics[width=.16\linewidth]{CVPR2021/supp/sidd_fig_10/box_cbdnet.PNG}  
  \includegraphics[width=.16\linewidth]{CVPR2021/supp/sidd_fig_10/box_ridnet.PNG} 
  \includegraphics[width=.16\linewidth]{CVPR2021/supp/sidd_fig_10/box_vdnet.PNG}  
  \includegraphics[width=.16\linewidth]{CVPR2021/supp/sidd_fig_10/box_danet.PNG}  
  \includegraphics[width=.16\linewidth]{CVPR2021/supp/sidd_fig_10/box_ours.PNG}
  % figure 10
%   \includegraphics[width=.16\linewidth]{CVPR2021/supp/sidd_fig_11/box_noisy.PNG} 
%   \includegraphics[width=.16\linewidth]{CVPR2021/supp/sidd_fig_11/box_cbdnet.PNG}  
%   \includegraphics[width=.16\linewidth]{CVPR2021/supp/sidd_fig_11/box_ridnet.PNG} 
%   \includegraphics[width=.16\linewidth]{CVPR2021/supp/sidd_fig_11/box_vdnet.PNG}  
%   \includegraphics[width=.16\linewidth]{CVPR2021/supp/sidd_fig_11/box_danet.PNG}  
%   \includegraphics[width=.16\linewidth]{CVPR2021/supp/sidd_fig_11/box_ours.PNG}
%   \caption{\textbf{DND~\cite{DND_2017_CVPR} visualization examples.} \ourmodel produces fewer fake dots, restores better colors and finer textures. }
  \label{fig:sub-first}
\end{subfigure}
\caption{Visualization results on the SIDD dataset of \ourmodel compared against other competitive models. Boxed regions are zoomed results. Best viewed in color on a high-resolution display. }
\label{fig:more_sidd}
\vspace{-6mm}
\end{figure*}

\begin{figure*}[t]
\centering
% Caption
\begin{subfigure}{.16\textwidth}
  \centering
  % include first image
  \caption*{Noisy} 
\end{subfigure}
\begin{subfigure}{.16\textwidth}
  \centering
  % include second image
  \caption*{CBDNet~\cite{Guo2019Cbdnet}} 
\end{subfigure}
\begin{subfigure}{.16\textwidth}
  \centering
  % include second image
  \caption*{RIDNet~\cite{RIDNet}} 
\end{subfigure}
\begin{subfigure}{.16\textwidth}
  \centering
  % include first image
  \caption*{VDN~\cite{VDN}}   
\end{subfigure}
\begin{subfigure}{.16\textwidth}
  \centering
  % include second image
  \caption*{DANet~\cite{DANet}} 
\end{subfigure}
\begin{subfigure}{.16\textwidth}
  \centering
  % include second image
  \caption*{\ourmodel (Ours)} 
\end{subfigure}
% SIDD
\begin{subfigure}{1.\textwidth} 
  \centering
  % figure 1
  \includegraphics[width=.16\linewidth]{CVPR2021/supp/dnd_fig_0/box_noisy.png} 
  \includegraphics[width=.16\linewidth]{CVPR2021/supp/dnd_fig_0/box_cbdnet.png} 
  \includegraphics[width=.16\linewidth]{CVPR2021/supp/dnd_fig_0/box_ridnet.PNG} 
  \includegraphics[width=.16\linewidth]{CVPR2021/supp/dnd_fig_0/box_vdnet.PNG}  
  \includegraphics[width=.16\linewidth]{CVPR2021/supp/dnd_fig_0/box_danet.PNG}  
  \includegraphics[width=.16\linewidth]{CVPR2021/supp/dnd_fig_0/box_ours.PNG} 
  % figure 2
  \includegraphics[width=.16\linewidth]{CVPR2021/secs/images/visual_13/box_noisy.png} 
  \includegraphics[width=.16\linewidth]{CVPR2021/secs/images/visual_13/box_cbdnet.png} 
  \includegraphics[width=.16\linewidth]{CVPR2021/secs/images/visual_13/box_ridnet.png}  
  \includegraphics[width=.16\linewidth]{CVPR2021/secs/images/visual_13/box_vdnet.png} 
  \includegraphics[width=.16\linewidth]{CVPR2021/secs/images/visual_13/box_danet.png} 
  \includegraphics[width=.16\linewidth]{CVPR2021/secs/images/visual_13/box_ours.png} 
  % figure 3
  \includegraphics[width=.16\linewidth]{CVPR2021/supp/dnd_fig_1/box_noisy.png} 
  \includegraphics[width=.16\linewidth]{CVPR2021/supp/dnd_fig_1/box_cbdnet.png} 
  \includegraphics[width=.16\linewidth]{CVPR2021/supp/dnd_fig_1/box_ridnet.PNG} 
  \includegraphics[width=.16\linewidth]{CVPR2021/supp/dnd_fig_1/box_vdnet.PNG}  
  \includegraphics[width=.16\linewidth]{CVPR2021/supp/dnd_fig_1/box_danet.PNG}  
  \includegraphics[width=.16\linewidth]{CVPR2021/supp/dnd_fig_1/box_ours.PNG}  
  % figure 4
  \includegraphics[width=.16\linewidth]{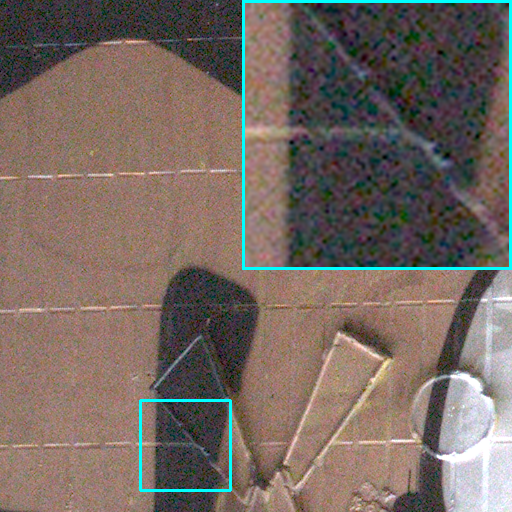} 
  \includegraphics[width=.16\linewidth]{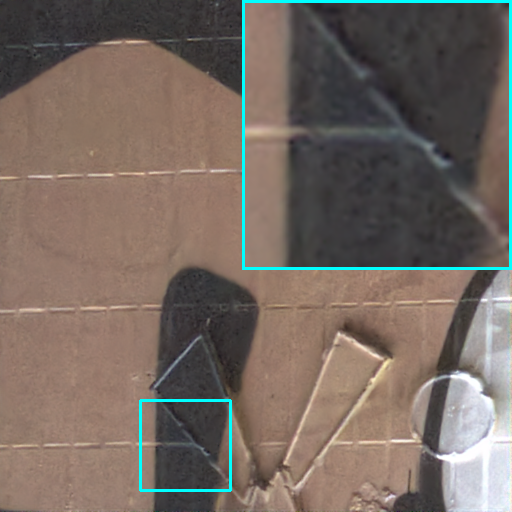}  
  \includegraphics[width=.16\linewidth]{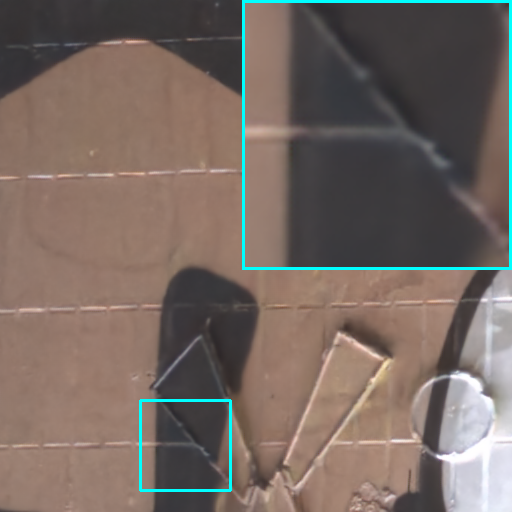} 
  \includegraphics[width=.16\linewidth]{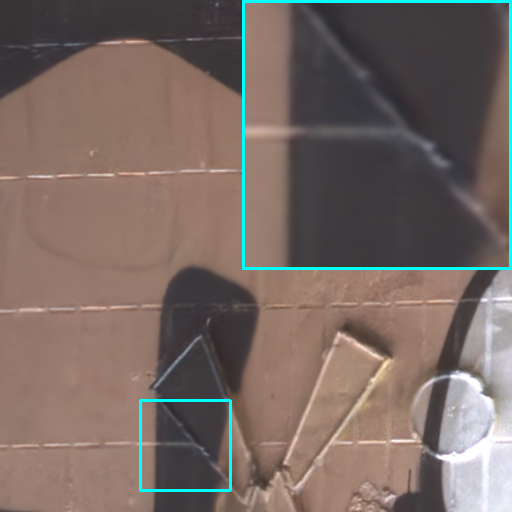}  
  \includegraphics[width=.16\linewidth]{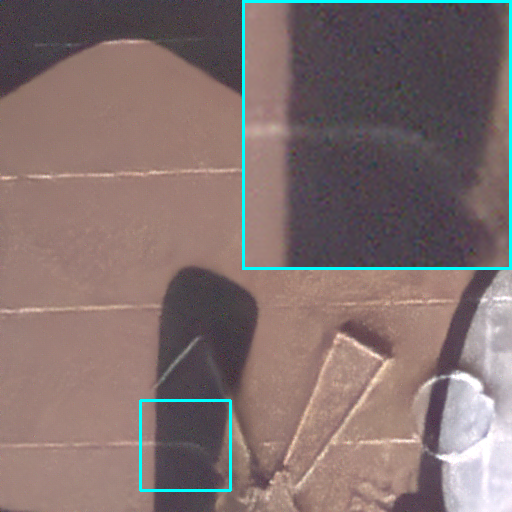}  
  \includegraphics[width=.16\linewidth]{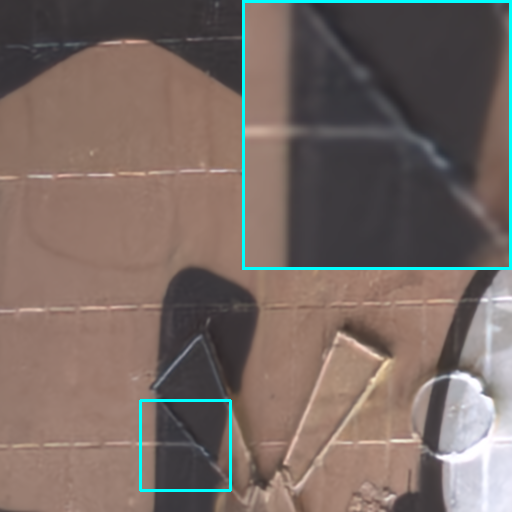}
  % figure 5
  \includegraphics[width=.16\linewidth]{CVPR2021/supp/dnd_fig_3/box_noisy.PNG} 
  \includegraphics[width=.16\linewidth]{CVPR2021/supp/dnd_fig_3/box_cbdnet.PNG}  
  \includegraphics[width=.16\linewidth]{CVPR2021/supp/dnd_fig_3/box_ridnet.PNG} 
  \includegraphics[width=.16\linewidth]{CVPR2021/supp/dnd_fig_3/box_vdnet.PNG}  
  \includegraphics[width=.16\linewidth]{CVPR2021/supp/dnd_fig_3/box_danet.PNG}  
  \includegraphics[width=.16\linewidth]{CVPR2021/supp/dnd_fig_3/box_ours.PNG}
  % figure 6
  \includegraphics[width=.16\linewidth]{CVPR2021/supp/dnd_fig_4/box_noisy.PNG} 
  \includegraphics[width=.16\linewidth]{CVPR2021/supp/dnd_fig_4/box_cbdnet.PNG}  
  \includegraphics[width=.16\linewidth]{CVPR2021/supp/dnd_fig_4/box_ridnet.PNG} 
  \includegraphics[width=.16\linewidth]{CVPR2021/supp/dnd_fig_4/box_vdnet.PNG}  
  \includegraphics[width=.16\linewidth]{CVPR2021/supp/dnd_fig_4/box_danet.PNG}  
  \includegraphics[width=.16\linewidth]{CVPR2021/supp/dnd_fig_4/box_ours.PNG}
  % figure 7
  \includegraphics[width=.16\linewidth]{CVPR2021/supp/dnd_fig_5/box_noisy.PNG} 
  \includegraphics[width=.16\linewidth]{CVPR2021/supp/dnd_fig_5/box_cbdnet.PNG}  
  \includegraphics[width=.16\linewidth]{CVPR2021/supp/dnd_fig_5/box_ridnet.PNG} 
  \includegraphics[width=.16\linewidth]{CVPR2021/supp/dnd_fig_5/box_vdnet.PNG}  
  \includegraphics[width=.16\linewidth]{CVPR2021/supp/dnd_fig_5/box_danet.PNG}  
  \includegraphics[width=.16\linewidth]{CVPR2021/supp/dnd_fig_5/box_ours.PNG}
%   \caption{\textbf{DND~\cite{DND_2017_CVPR} visualization examples.} \ourmodel produces fewer fake dots, restores better colors and finer textures. }
  \label{fig:sub-first}
\end{subfigure}
\caption{Visualization results on the DND dataset of \ourmodel compared against other competitive models. Boxed regions are zoomed results. Best viewed in color on a high-resolution display. }
\label{fig:more_dnd}
\vspace{-6mm}
\end{figure*}
